# Supplementary material for: Bayesian calibration and sensitivity analysis for a karst aquifer model using active subspaces
Source: arXiv:1901.03283 source file (2019-07-16)
Supplement: Supplementary file 1 [file main_supp_info.pdf]

# Supporting Information for *Bayesian calibration and sensitivity analysis for a karst aquifer model using active subspaces*

Mario Teixeira Parente<sup>1</sup>, Daniel Bittner<sup>2</sup>, Steven A. Mattis<sup>1</sup>, Gabriele

Chiogna<sup>2,3</sup>, Barbara Wohlmuth<sup>1</sup>

<sup>1</sup>Chair for Numerical Mathematics, Technical University Munich, Boltzmannstraße 3, 85748 Garching near Munich, Germany

<sup>2</sup>Chair of Hydrology and River Basin Management, Technical University Munich, Arcisstraße 21, 80333 Munich, Germany

<sup>3</sup>Institute of Geography, University of Innsbruck, Innrain 52, 6020 Innsbruck, Austria

## Contents of this file

1. Figures S1 to S3

## Introduction

The supporting information comprises three figures that are said to support the scientific content provided in the main text. Fig. S1 gives an overview about the natural characteristics of the study area in Waidhofen a.d. Ybbs. The orthophoto in Fig. S1a), taken in 2006, was kindly provided by the water works owner in Waidhofen. The shown recharge area of the Kerschbaum spring was mapped by Hacker (2003). Fig. S2 is taken from Bittner, Narany, Kohl, Disse, and Chiogna (2018) to provide visual help for the LuKARS model and the interconnection of different hydrotopes. Fig. S3 provides a visual overview of the input data processed to run the Kerschbaum LuKARS model. The daily temperature was used in the temperature index snow model (Martinec, 1960) as

---

well as to calculate evapotranspiration (Thornthwaite, 1948). The precipitation time series was processed as an input for LuKARS and the discharge time series was used to calibrate the LuKARS model. All input data was kindly provided by the water works Waidhofen a.d. Ybbs.

## References

- Bittner, D., Narany, T. S., Kohl, B., Disse, M., & Chiogna, G. (2018). Modeling the hydrological impact of land use change in a dolomite-dominated karst system. *Journal of Hydrology*, 567, 267–279.
- GBA. (2018). *Geologische Bundeslnderkarten, Geologische Bundesanstalt sterreich*. [https://gisgba.geologie.ac.at/arcgis/services/image/AT\\_GBA\\_GK100\\_200/ImageServer/WMSServer?request=GetCapabilities&](https://gisgba.geologie.ac.at/arcgis/services/image/AT_GBA_GK100_200/ImageServer/WMSServer?request=GetCapabilities&). (April 18th, 2018)
- Hacker, P. (2003). Hydrologisch-hydrogeologische Untersuchungen im Bereich des Glashüttenberges zur Frage des engeren Schutzgebietes für die Kerschbaumer-Quelle. *ARC Seibersdorf research GmbH*.
- Martinec, J. (1960). The degree-day factor for snowmelt runoff forecasting. *IUGG General Assembly of Helsinki, IAHS Commission of Surface Waters*, 51, 468–477.
- Thornthwaite, C. W. (1948). *An approach toward a rational classification of climate* (Vol. 66) (No. 1). LWW.

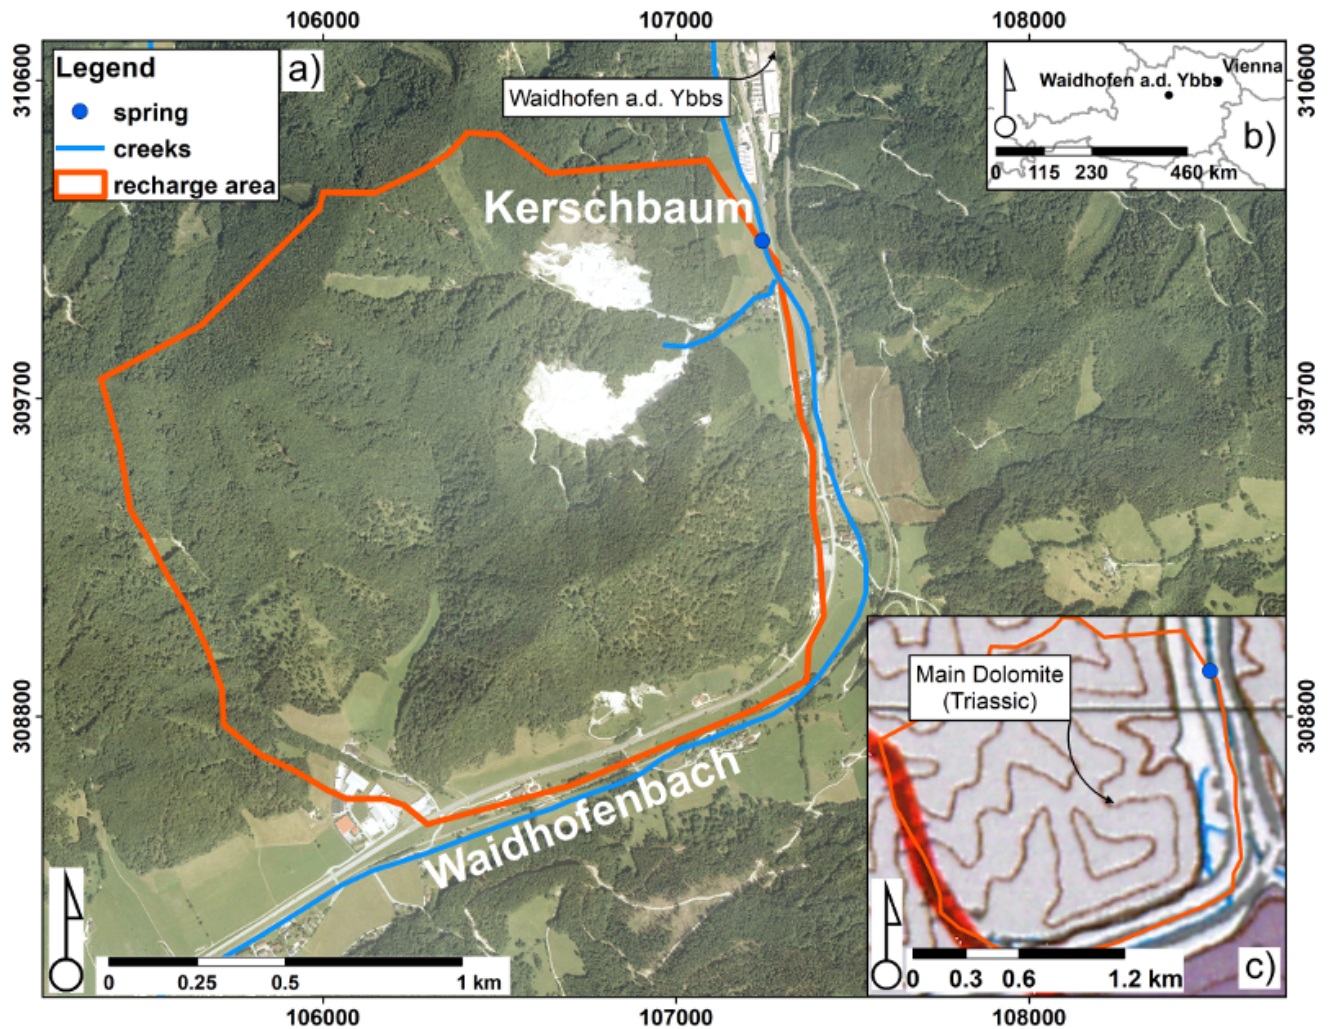

**Figure S1.** Overview of the characteristics of the Kerschbaum spring recharge area and its geographical localization. a) an orthophoto and the boundary of the recharge area with the location of the Kerschbaum spring. b) the geographical position of Waidhofen a.d. Ybbs in Austria. c) the dominant presence of dolomitic basement rocks in the catchment (GBA, 2018). The isolines represent different elevation levels.

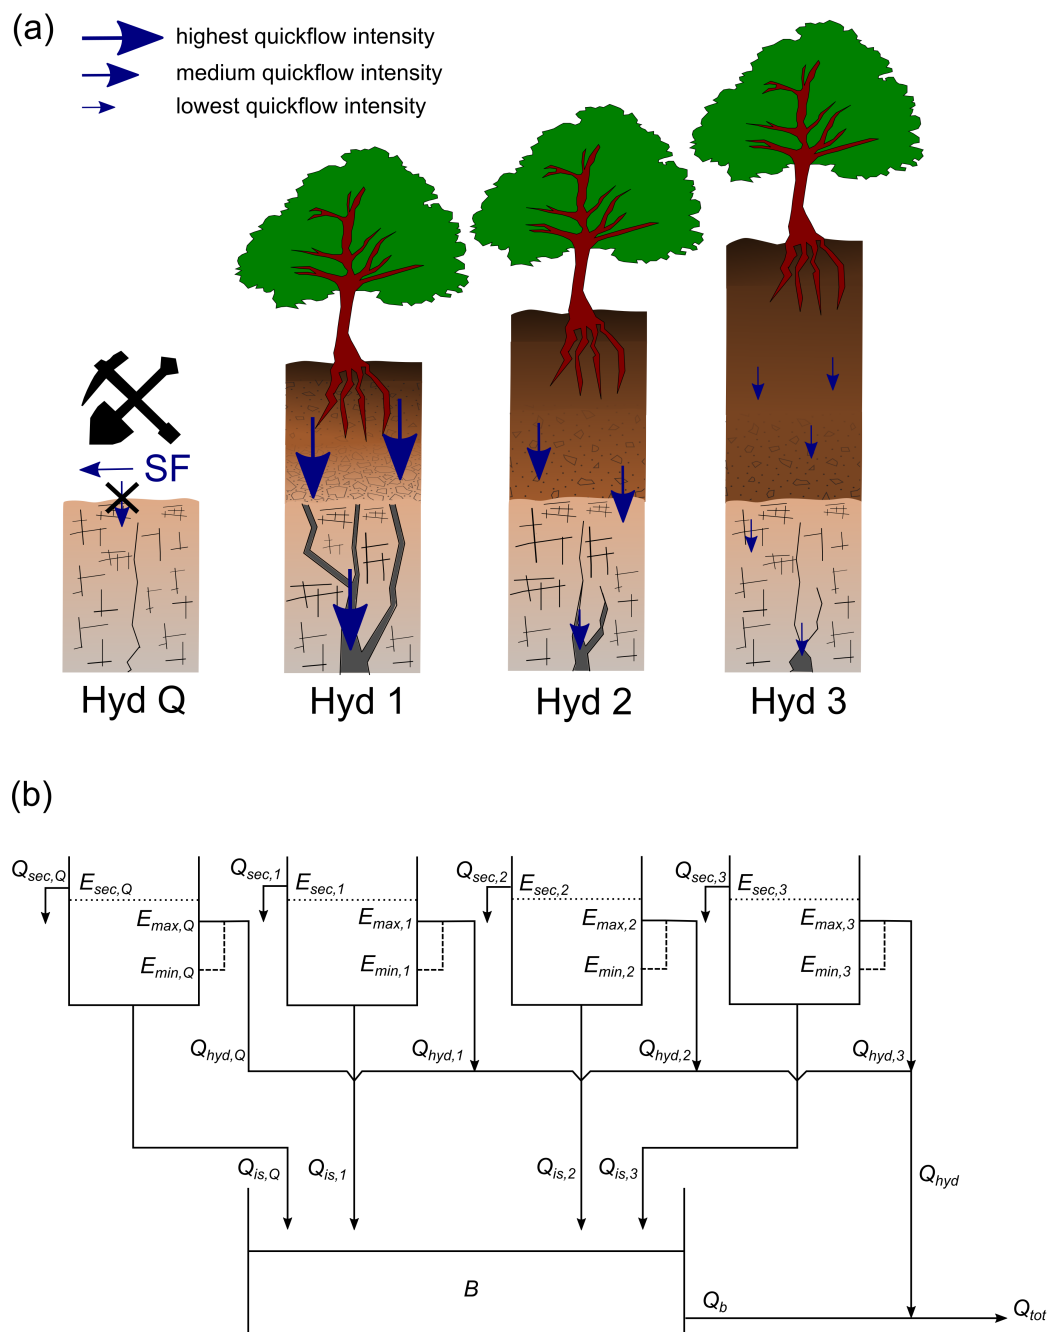

**Figure S2.** Conceptual sketch of the LuKARS model structure as provided in Bittner et al. (2018). Hyd Q represents the dolomite quarries, where no infiltration occurs due to a compacted protection layer and all water is drained by surface flow. The figure highlights the decreasing quickflow intensity from Hyd 1 to Hyd 3 due to the increasing soil depth and increasing content of fine-textured soil.

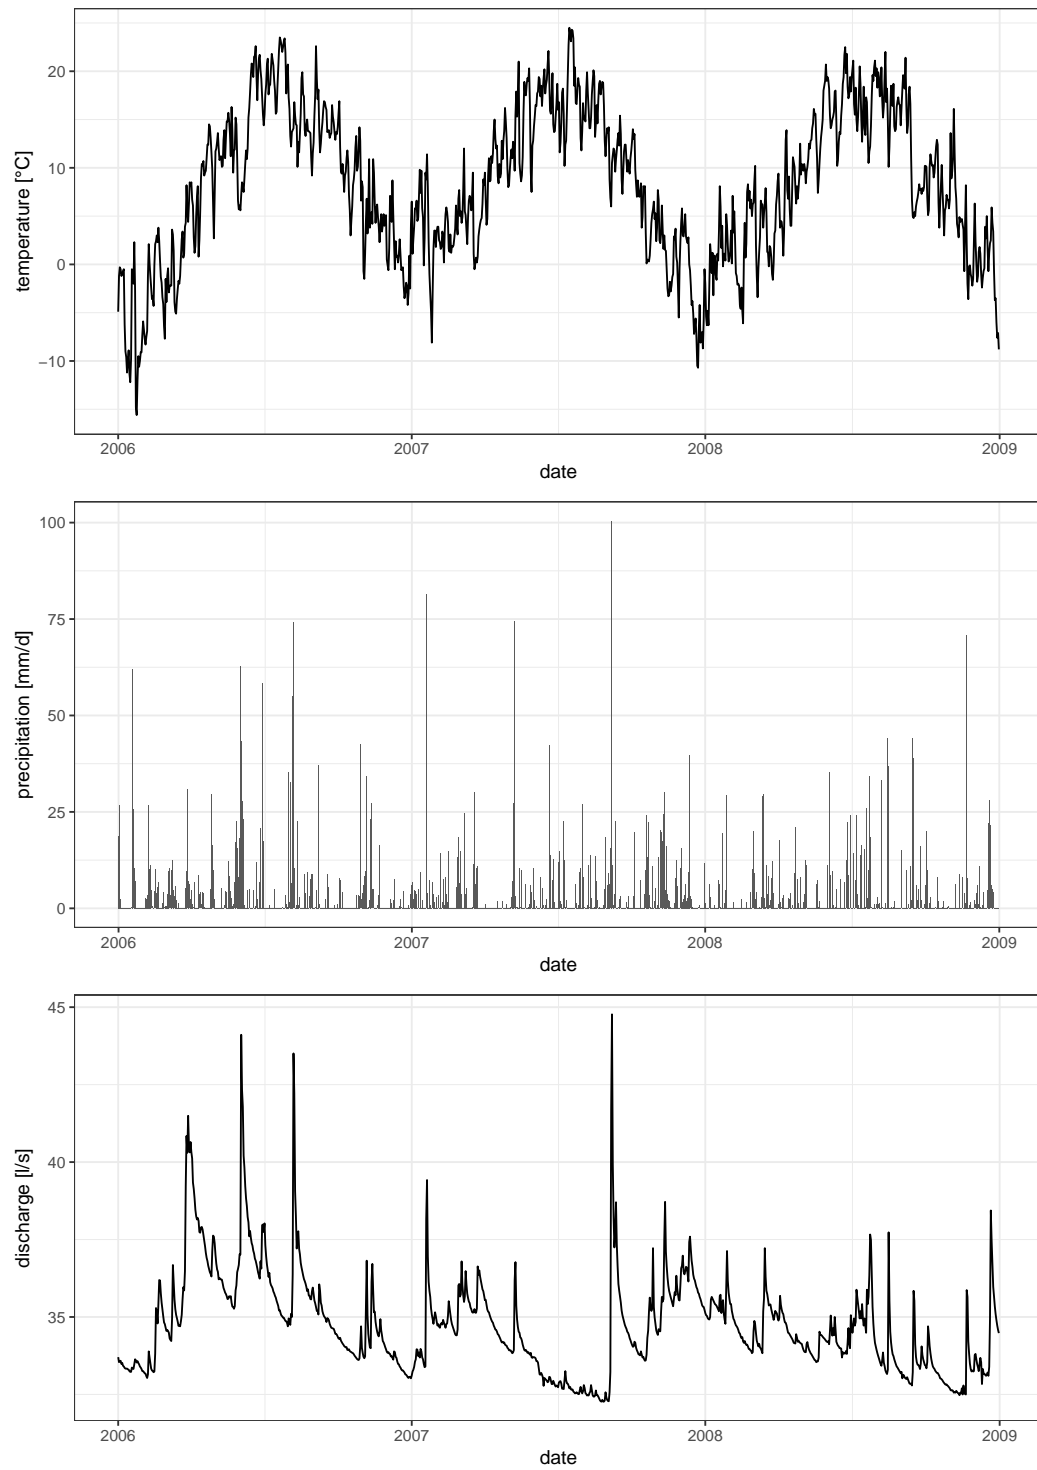

**Figure S3.** Input data used to run the LuKARS model, including daily temperature (top), daily precipitation (middle), and daily discharge values of the Kerschbaum spring (bottom).

May 8, 2019, 8:37am
